# Supplementary material for: Relative Representations Enable Portable White-Box Monitoring Across Language Models
Source: arXiv:2610.28366 source file (2026-10-20)
Supplement: Supplementary file 1 [file full_related_work.tex]

\section{Comprehensive related work}
\label{app:rel-work}

\subsection{White-box probing of language models}

Linear probes and diagnostic classifiers show that model representations
contain decodable syntactic and semantic structure
\citep{Conneau2018-cram, Tenney2019-bert-pipeline}, spatial and temporal
information \citep{Gurnee2023-space-time}, and broad behavioral traits
\citep{Zou2023-rep-engineering}. Internal-state monitors have been used to
anticipate answer quality and model behavior
\citep{Ferrando2024-do-i-know, Gottesman2024-estimating-knowledge,
Joshi2024-personas-truthfulness, Afzal2025-knowing-before-saying}, detect
factual errors and hallucinations
\citep{CH-Wang2023-electric-sheep, Chen2024-inside, Orgad2024-zp,
Simhi2024-combating-hallucinations, Snyder2024-early-hallucinations}, and
identify safety-relevant inputs or behavior
\citep{McKenzie2026-su, Kramar2026-zv}. These studies establish that useful
monitoring targets are present in model activations.

Probe performance does not by itself establish a robust or portable monitor.
Prior work documents methodological pitfalls
\citep{Hewitt2019-control-tasks, Voita2020-mdl-probing,
Belinkov2022-probing-survey}, failures under task and distribution shifts
\citep{Levinstein2023-no-lie-detector, Kramar2026-zv, Min2026-corvus}, and
sensitivity to probe-layer choice \citep{Mallen2023-gs}. \citet{Liang2025-neural-probe}
address this sensitivity by using Bayesian optimization to select a single
probe insertion layer. A probe is also expressed in the native activation
coordinates of its host model. Applying the learned coefficients to another
model generally fails or is undefined when dimensions differ.

Several architectures aggregate information across transformer layers within
one model \citep{Suresh2025-clap, Nordby2026-multilayer,
Huang2026-deepguard}. These methods support the view that monitoring
information can be distributed across the residual stream. Our global
representation also uses all transformer layers. It then converts the
whole-network activation into a fixed anchor-indexed vector, which allows the
same fitted probe to be evaluated across models.

\subsection{Relative representations and representational convergence}

\citet{Moschella2022-es} introduce relative representations based on
similarities to a fixed anchor set. Their construction removes nuisance
variation under latent isometries and rescalings and enables zero-shot
communication among latent spaces from different training runs and
architectures. They demonstrate component reuse for classification and
reconstruction. This establishes that anchor-relative coordinates can support
transferable downstream computation.

Our work applies the same general construction to residual-stream states of
autoregressive language models. The targets are behavioral properties of the
model's own answer or completion. We use a whole-network profile, transfer a
frozen post-hoc probe across independently trained model families, and study
scale, learned updates, prompts, and data shifts. The blinded correspondence
analysis asks whether the shared anchor ordering can be partially recovered
from the two models' geometry.

Model stitching also tests functional compatibility between representations
\citep{Bansal2021-model-stitching}. Stitching methods insert a trained bridge
between two model components. Our anchor-relative coordinates are fixed by
shared examples and require no learned source--target bridge.

The Platonic Representation Hypothesis proposes that models increasingly agree
on similarity structure as their capability and coverage improve
\citep{Huh2024-platonic}. Indra representations describe each sample by its
angular distances to the other samples and improve robustness of downstream
classifiers and cross-modal retrieval \citep{Lu2025-indra}. They do not
consider probe transfer across models, and construct full distance profiles
over a dataset rather than using a fixed set of common anchors. A full Indra
profile has quadratic cost in the number of samples, whereas an anchor set gives a
finite relational profile whose dimension is chosen independently of the
evaluation-set size. Our study tests whether relational compatibility extends
to information about an autoregressive language model's own behavior.

\subsection{Cross-model monitoring and activation transfer}

ACT-ViT directly studies cross-model white-box monitoring
\citep{Bar-Shalom2025-ig}. It processes activation tensors using pooling, a
linear adapter for each language model, and a shared vision-transformer
backbone pretrained on labeled activations from multiple model--dataset pairs.
The adapter maps each model's hidden dimension into that shared backbone, so
extending the system to a new model requires fitting a new model-specific
adapter. Our method instead computes a fixed anchor-relative representation and
applies a lightweight frozen probe after an unlabeled anchor pass.

\citet{oozeer2025activationspaceinterventionstransferred} study transfer of
safety interventions through learned source--target activation mappers. Their
autoencoder and affine mappings are model-pair-specific and are evaluated for
intervention transfer. Our setting concerns monitoring and uses a shared
anchor-indexed coordinate system. These approaches address adjacent questions
about how activation-space tools can operate across models.

\citet{Obeso2025-ns} evaluate a different form of cross-model generalization.
A probe hosted on model $A$ detects hallucinations in text generated by model
$B$, while the generated text is passed through model $A$ to obtain the
activations. The probe remains in its host activation space. This setup incurs
an additional forward pass through the monitoring model. Our probes operate on
the generating model's own activations, after the probe has been transferred
from a source model.
